# Supplementary material for: Low-Loss High-Fidelity Frequency-Mode Hadamard Gates Based on Electromagnetically Induced Transparency
Source: arXiv:1907.03393 ancillary file (2019-08-14)
Supplement: Supplementary file 1 [file Supplemental_Material.pdf]

# SUPPLEMENTAL MATERIAL

## Low-Loss High-Fidelity Frequency-Mode Hadamard Gates Based on Electromagnetically Induced Transparency


Kao-Fang Chang[1], Ta-Pang Wang[1], Chun-Yi Chen[1], Yi-Hsin Chen[2,5], Yu-Sheng Wang[1], Yong-Fan Chen[3,5,*], Ying-Cheng Chen[4,5], and Ite A. Yu[1,5,*]

[1]*Department of Physics, National Tsing Hua University, Hsinchu 30013, Taiwan*

[2]*Department of Physics, National Sun Yat-sen University, Kaohsiung 80424, Taiwan*

[3]*Department of Physics, National Cheng Kung University, Tainan 70101, Taiwan*

[4]*Institute of Atomic and Molecular Sciences, Academia Sinica, Taipei 10617, Taiwan*

[5]*Center for Quantum Technology, Hsinchu 30013, Taiwan*


## I. EXPERIMENTAL SYSTEM

The cold $^{87}$Rb atoms in the experiment were produced by a magneto-optical trap (MOT). There were about $3 \times 10^9$ in the cigar-shaped atom cloud of the dimension of $14{\times}2{\times}2$ mm$^{-3}$ [1]. Before each measurement, we optically pumped all population to the Zeeman states of $|F = 1, m = 1\rangle$ and $|F = 2, m = 2\rangle$ [2]. The population in $|F = 2, m = 2\rangle$ is irrelevant to this study, and all laser fields in the FWM measurement did not drive this state. Figure 1(a) shows the transitions driven by the probe, coupling, driving, and signal fields, all of which had the $\sigma+$ polarization, and propagated along the major axis of the atom cloud. The optical depth (OD) of the probe and signal transitions was about 100$\sim$130. The wavelength of the probe and coupling fields is 780 nm, and that of the driving and signal fields is 795 nm. We used light from a master laser to seed the probe and coupling lasers for the stabilization of frequency difference between the two lasers [3]. An electro-optic modulator (EOM) was installed in one of the seeding paths. The first-order sideband of the EOM was employed for the seeding, which produces a frequency difference of about 6.8 GHz between the probe and coupling lasers. We made the similar arrangement to seed the signal and driving lasers. Therefore, the decoherence rate caused by fluctuation of the frequency difference between the probe and coupling fields (or between the signal and driving fields) was little.

The coupling and driving beams came out of a polarization-maintained (PM) optical fiber before entering the atom cloud, and the probe and signal beams came out of another PM optical fiber. This can ensure the coupling and driving beams (the probe and signal beams) to spatially-overlap well. The $e^{-2}$ full width of the coupling and driving beams was 2.0 mm, and that of the probe and signal beams was 0.2 mm. We arranged an angle separation of about 0.9° between the coupling (driving) and the probe (signal) propagation directions. This angle separation is small enough to make negligible decoherence rate [4, 5], and is also large enough to prevent the coupling and driving light from entering the probe's and signal's SPCMs.

A scheme of spatial filter was also used to block the coupling and driving light. In Fig. 1(b), the coupling and driving beams first passed through F200-1 before merged with the probe and signal beams at NBS, then became quasi-plane waves after F175, and finally were focused by F200-2 and blocked by BB at the focal point. The probe and signal beams were focused to the center of the atom cloud by F175, and transformed to quasi-plane waves by F200-2. Because of the angle separation, BB which is actually an iris diaphragm caused little attenuation of the probe and signal light.

Several technical issues involved in the low-loss FWM process. First of all, a medium's OD ($\alpha$) must be sufficiently large. The conversion efficiency from one wavelength to another can be enhanced by OD, shown by Eq. (S6) in Sec. III. A larger OD can also make the 50/50 FBS have a higher total transmission and a better fidelity as illustrated in Subsection III B of the Supplemental Material. Secondly, the wavelength conversion process requires the phase match, i.e., $\Delta k \equiv (\vec{k}_p - \vec{k}_c + \vec{k}_d - \vec{k}_s)\cdot\hat{z} = 0$ where $\vec{k}_x$ represents the wave vector of light field. A phase mismatch, i.e., $\Delta k \neq 0$, can cause the loss. For example, the propagation directions of 780 nm coupling and probe (or 795 nm driving and signal) beams have an angle separation of about 0.9°, resulting in $L\Delta k = 0.23$ radians in our system, where $L$ is the medium length, and a loss of 6%. Fortunately, our study showed that a suitable two-photon detuning ($\delta$) can compensate the phase mismatch. The experimental and theoretical studies of using $\delta$ to compensate a phase mismatch will be published elsewhere. Finally and most importantly, the efficiency of FWM process is sensitive to the ground-state decoherence rate ($\gamma$) [6]. Thus, $\gamma$ must be as low as possible. The decoherence can be caused by stray magnetic fields in the transverse direction, frequency fluctuations of the two-photon Raman transition, inhomogeneity of the AC Stark shift, inhomogeneity of the longitudinal magnetic field, etc. Our works on the reduction of $\gamma$ can be found in Ref. [3]. In our system, $\gamma$ was


*yu@phys.nthu.edu.tw; yfchen@mail.ncku.edu.tw

mainly due to an unwanted but unavoidable transition of $|5S_{1/2}, F=2\rangle \rightarrow |5P_{3/2}, F'=3\rangle$ driven by the coupling field with a large detuning of 266 MHz or about 44Γ [7, 8], where Γ is the spontaneous decay rate of the excited state.

## II. THEORETICAL CALCULATION

To characterize our experimental system and verify measurement outcomes, we made theoretical predictions with the optical Bloch equations (OBEs) of density-matrix operator and the Maxwell-Schrödinger equations (MSEs) of light fields given below [9, 10].

$$\frac{\partial}{\partial t}\rho_{21} = \frac{i}{2}\Omega_c^*\rho_{31} + \frac{i}{2}\Omega_d^*\rho_{41} + i\delta\rho_{21} - \gamma\rho_{21}, \quad \text{(S1)}$$

$$\frac{\partial}{\partial t}\rho_{31} = \frac{i}{2}\Omega_p + \frac{i}{2}\Omega_c\rho_{21} - \frac{\Gamma}{2}\rho_{31}, \quad \text{(S2)}$$

$$\frac{\partial}{\partial t}\rho_{41} = \frac{i}{2}\Omega_s + \frac{i}{2}\Omega_d\rho_{21} + i\Delta\rho_{41} - \frac{\Gamma}{2}\rho_{41}, \quad \text{(S3)}$$

$$\frac{1}{c}\frac{\partial}{\partial t}\Omega_p + \frac{\partial}{\partial z}\Omega_p = i\frac{\alpha}{2L}\Gamma\rho_{31}, \quad \text{(S4)}$$

$$\frac{1}{c}\frac{\partial}{\partial t}\Omega_s + \frac{\partial}{\partial z}\Omega_s = i\frac{\alpha}{2L}\Gamma\rho_{41}, \quad \text{(S5)}$$

where $\rho_{ij}$ is the element of density matrix operator of states $|i\rangle$ and $|j\rangle$, $\Omega_c$, $\Omega_d$, $\Omega_p$, and $\Omega_s$ are the Rabi frequencies of the coupling, driving, probe, and signal fields, $\delta$ is the two-photon detuning of the Raman transitions between two ground states $|1\rangle$ and $|2\rangle$, $\Delta$ is the one-photon detuning of the transition $|1\rangle \rightarrow |4\rangle$ or $|2\rangle \rightarrow |4\rangle$, $\gamma$ is the ground-state decoherence rate, $\Gamma$ is the spontaneous decay rate of the excited states $|3\rangle$ and $|4\rangle$ which is about $2\pi\times6$ MHz in the experiment, and $\alpha$ and $L$ are the optical depth (OD) and length of the medium. To achieve the above equations, we consider that the probe and signal fields are weak and can be treated as the perturbations of the system. The excited states $|3\rangle$ and $|4\rangle$ belong to the $D2$ and $D1$ lines of Rb atoms. The spontaneous decay rates of $|3\rangle$ and $|4\rangle$ as well as the transition strengths of $|1\rangle \rightarrow |3\rangle$ and $|1\rangle \rightarrow |4\rangle$ differ by about 5.3%. In the theoretical calculation, we set the same decay rate for $\rho_{31}$ and $\rho_{41}$, and used the same OD for the probe and signal transitions. Since we always tuned the probe and coupling frequencies to the resonance frequencies of their transitions in the experiment, no one-photon detuning is present in Eq. (S2).

## III. DETERMINATION OF EXPERIMENTAL PARAMETERS

We employed the measurement of slow light to determine the coupling Rabi frequency $\Omega_c$. A typically data of slow light of the probe pulse under the presence of the coupling field is shown in Fig. S1(a). According to the theory or theoretical predictions calculated with the OBEs and MSEs in Eqs. (S1), (S2) and (S4), the delay time of slow light is equal to $\alpha\Gamma/\Omega_c^2$ [1, 11]. Once the OD ($\alpha$) is known which will be explained in the next paragraph, we can determine $\Omega_c$ from the delay time between input and output probe pulses. Attenuation of the probe pulse can be utilized to determine the decoherence rate $\gamma$, which was about $3\times10^{-3}\Gamma$ or $2\pi\times18$ kHz in this work. Furthermore, the condition of the coupling and driving fields having the same Rabi frequencies, i.e.,

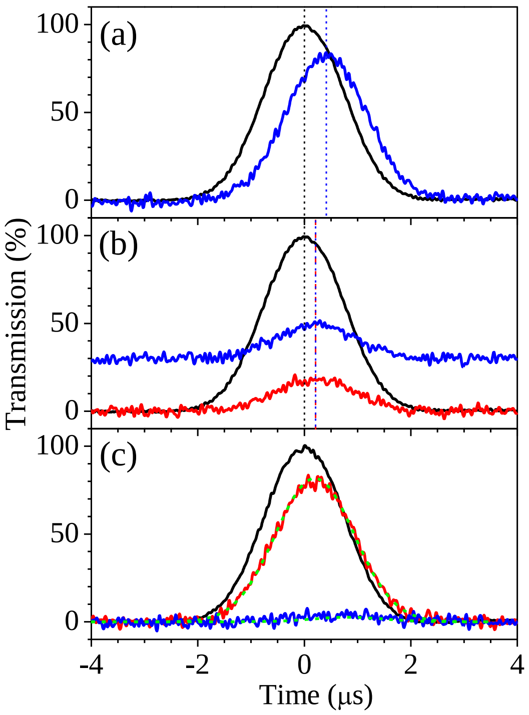


FIG. S1: Data of slow light in the single-Λ and double-Λ systems are shown in (a) and (b), respectively. Data of coherent wavelength conversion are presented in (c). In all of the data here, only the 780 nm probe pulse was sent to the input represented by black solid lines. Blue and red solid lines are the 780 nm probe and 795 nm signal pulses at the output. (a) Slow light of the probe pulse under the presence of only the coupling field. (b) Slow light of the probe and signal pulses under the presence of both of the coupling and driving fields at $\Delta = 0$. Blue line is shifted up for clarity. The coupling Rabi frequencies in (a) and (b) were the same. Thus, the delay time in (b) became half of that in (a), indicating the coupling and driving fields had the same Rabi frequency, i.e., $\Omega_c = \Omega_d$. (c) At $\Delta/(2\pi) = -135$ MHz and $\Omega_c = \Omega_d$, the FWM process converted the input probe pulse nearly all to the output signal pulse. The 795 nm output transmission (ratio of output to input energies or photon numbers) was about 83%, and the 780 nm one was less than 4%. In (c), green dashed lines are the theoretical predictions calculated with $\alpha$ (OD) = 130, $\Omega_c = \Omega_d = 3.0\Gamma$, and $\gamma$ (the ground-state decoherence rate) = $3\times10^{-3}\Gamma$. The values of $\alpha$, $\Omega_c$ ($\Omega_d$), and $\gamma$ were experimentally determined by the optimum one-photon detuning $\Delta_{\rm opt}$ that maximizes the output signal pulse, the delay times in (a) and (b), and the ratio of output to input pulse amplitudes in (a), respectively.

$\Omega_c = \Omega_d$, was needed thorough all measurements of this work. We not only ensured $\Omega_c = \Omega_d$ by monitoring the powers of the coupling and driving fields, but also verified $\Omega_c = \Omega_d$ with the measurement of resonant FWM process (i.e., $\Delta = 0$) as shown in Fig. S1(b). In the resonant FWM process, only the probe pulse was sent to the input, and both of the coupling and driving fields were present. From the theory or theoretical predictions calculated with the OBEs and MSEs in Eqs. (S1)-(S5), the delay time in the resonant FWM process is equal to $\alpha\Gamma/(\Omega_c^2 + \Omega_d^2)$ [2, 10]. As the delay time in Fig. S1(b) became half of that in Fig. S1(a), we can know that $\Omega_d = \Omega_c$ and two fields have the same Rabi frequencies.

To determine the OD ($\alpha$) of the experimental system, we employed the measurement of far-detuned FWM process, i.e., $|\Delta| \gg \Gamma$. In the far-detuned FWM process, only the probe pulse was sent to the input, and we measured the signal pulse at the output. In the measurement, we set $\Omega_c = \Omega_d$. The driving field had the one-photon detuning $\Delta$. According to the steady-state solution of Eqs. (S1)-(S5), the ratio of output signal (probe) field to input probe field under $\gamma = 0$ is given by [9]

$$\frac{|\Omega_s(z=L)|^2}{|\Omega_p(z=0)|^2} = \frac{1}{4}\left(1 + e^{-2A} - 2e^{-A}\cos\theta\right), \quad \text{(S6)}$$

$$\frac{|\Omega_p(z=L)|^2}{|\Omega_p(z=0)|^2} = \frac{1}{4}\left(1 + e^{-2A} + 2e^{-A}\cos\theta\right), \quad \text{(S7)}$$

where

$$\theta = \frac{\alpha}{2}\frac{\Delta/\Gamma}{1+(\Delta/\Gamma)^2}, \quad \text{(S8)}$$

$$A = \frac{\alpha}{2}\frac{1}{1+(\Delta/\Gamma)^2} = \frac{\alpha - \sqrt{\alpha^2 - 16\theta^2}}{4}. \quad \text{(S9)}$$

We now derive the criterion, which maximizes $|\Omega_s(L)|^2$ or equivalently minimizes $|\Omega_p(L)|^2$. Since Eq. (S6) or (S7) is a function of only $\alpha$ and $\Delta$, the OD of the system must be related to the optimum one-photon detuning $\Delta_{\rm opt}$ at the maximum. Given $\Delta_{\rm opt}$, we first take the derivative of Eq. (S6) with respect to $\alpha$, and obtained the criterion given by

$$-e^{-A}\frac{dA}{d\alpha} + \cos\theta\frac{dA}{d\alpha} + \sin\theta\frac{d\theta}{d\alpha} = 0. \quad \text{(S10)}$$

The value of $\alpha$ in the experiment was large as compared with $\theta$, which is close to $\pi$ at $\Delta_{\rm opt}$. Under $\alpha^2 \gg 16\theta^2$, $A \approx 2\theta^2/\alpha$. Because $A$ is small and $\theta \approx \pi$, we then make the approximations of $e^{-A} \approx 1 - A$, $\cos\theta \approx -1$, and $\sin\theta = \sin(\pi - \theta) \approx \pi - \theta$. After $\theta$ and $A$ are substituted by the expressions in Eqs. (S8) and (S9), the criterion finally becomes

$$\alpha \approx 2\pi|\Delta_{\rm opt}/\Gamma| - 4. \quad \text{(S11)}$$

Using the above equation and Eq. (S8), we also get $\theta \approx \pi - 2|\Gamma/\Delta_{\rm opt}|$. On the other hand, the numerical calculations using Eqs. (S1)-(S5) with all possible experimental parameters in this work also conclude a formula of $\alpha \approx 6.2|\Delta_{\rm opt}/\Gamma| - 6$ with an uncertainty of $\pm 4\%$. The value of $\alpha$ given by Eq. (S11) is consistent with that given by the numerical calculation. Therefore, by experimentally searching for $\Delta_{\rm opt}$ we can determine the OD of the system. As an example, Fig. S1(c) shows the output signal pulse was maximized at $\Delta_{\rm opt}/(2\pi) = -135\pm5$ MHz. The measured $\Delta_{\rm opt}$ indicates that the value of OD was 130±10 in Fig. S1(c).

## IV. A 50/50 FBS OPERATING WITH CLASSICAL LIGHT PULSES

We properly adjusted the one-photon detuning ($\Delta$) to produce a 50/50 FBS. Figure S2(a) shows the representative data that the 780 nm input pulse is split into the 780 nm and 795 nm output pulses of the very similar amount. At the split ratio of 0.48∼0.51, the average of data of output-to-input ratios or total transmissions taken in different days gave 89±4%, where the uncertainty is the standard deviation of the data. The values of OD in these measurements varied from 100 to 130. Furthermore, we performed the measurement that only the 795 nm signal pulse was present at the input under the same experimental condition as Fig. S2(a). The total transmission of 93±2% with the split ratio of 0.37∼0.46 was obtained, where the split ratio here is the ratio of 780 nm output energy to total output energy. The representative data are shown in Fig. S2(b). With the same 50/50 FBS, the outcomes of the 780 nm input differ from those of the 795 nm input, being caused by the non-negligible decoherence rate in the system and the asymmetry between the $D1$ and $D2$ excited states. The output-to-input ratio or overall efficiency presented here, which accounts for the input coupling efficiency, attenuation due to propagation in the medium, and frequency conversion efficiency, is the best up-to-date record of FBS.

## V. FIDELITY OF FREQUENCY BEAM SPLITTER

In analogy to an ordinary BS, 780 nm (or 795 nm) input photons are reflected into 795 nm (or 780 nm) output photons and transmitted into 780 nm (795 nm) output photons by the FBS, with the split ratio defined by the ratio of reflected output photon number to total output photon number. The fidelity $F$ is the important issue and can be determined by the following formula [12–14]:

$$F = \frac{\left|{\rm Tr}\left[\hat{V}^\dagger\hat{U}\right]\right|^2}{4T}, \quad \text{(S12)}$$

where $\hat{U}$ represents the operator of the ideal BS, $\hat{V}$ represents that of the FBS in this study, Tr[...] means the operation of trace, and $T$ is the total transmission of $\hat{V}$.

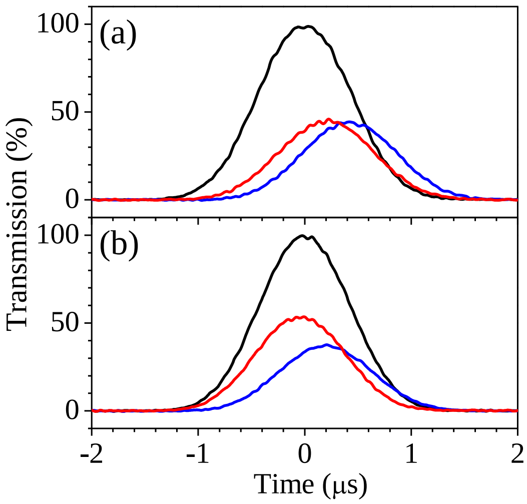


FIG. S2: A 50/50 frequency beam splitter operating with classical pulses. (a) At $\Delta/(2\pi) = -205$ MHz, $\alpha$ (OD) = 110, and $\Omega_c = \Omega_d = 3.0\Gamma$, the FWM process converted the input 780 nm probe (black) pulse to the output 795 nm signal (red) and 780 nm probe (blue) pulses with the transmissions of 46% and 45%, respectively. The delay time between the red (or blue) and black lines is 0.21 (or 0.42) $\mu$s. (b) Under the same experimental condition, the FWM process converted the input 795 nm (black) pulse to the output 795 nm (red) and 780 nm (blue) pulses with the transmissions of 53% and 38%, respectively. The delay time between the red (or blue) and black lines is $-0.04$ (or 0.20) $\mu$s.

One can write down the general expression of a FBS as

$$\hat{V} = \begin{bmatrix} t_1 & r_2 e^{i\phi_2} \\ r_1 e^{i\phi_1} & t_2 \end{bmatrix}, \tag{S13}$$

where $t_1$ (or $t_2$) and $r_1$ (or $r_2$) are the transmission and reflection coefficients of input 1 (or input 2), and $\phi_1$ (or $\phi_2$) is the phase difference between the reflected and transmitted outputs. Because of loss, $t_1^2 + r_1^2 \leq 1$ and $t_2^2 + r_2^2 \leq 1$. The split ratio of two inputs are determined by $r_1^2/(t_1^2 + r_1^2)$ and $r_2^2/(t_2^2 + r_2^2)$, and can be in general different.

### A. Frequency Beam Splitter with Tunable Split Ratio

We consider the case that the ground-state decoherence rate in the system is negligible, i.e., $\gamma = 0$. The steady-state solution of Eqs. (S1)-(S5) under $\Omega_c = \Omega_d$ provides $t_1$, $r_1$, $\phi_1$, $t_2$, $r_2$ and $\phi_2$ for $\hat{V}$ of the FWM-based FBS, which is given by

$$\hat{V} = \frac{1}{2}\begin{bmatrix} V_{11} & V_{12} \\ V_{21} & V_{22} \end{bmatrix}, \tag{S14}$$

where

$$V_{11} = V_{22} = \sqrt{1 + e^{-2A} + 2e^{-A}\cos\theta}, \tag{S15}$$

$$V_{12} = V_{21} = e^{i\phi/2}\sqrt{1 + e^{-2A} - 2e^{-A}\cos\theta}, \tag{S16}$$

$$A = \frac{\alpha - \sqrt{\alpha^2 - 16\theta^2}}{4}, \tag{S17}$$

$$\phi = 2\tan^{-1}\left(\frac{2e^{-A}}{1 - e^{-2A}}\sin\theta\right). \tag{S18}$$

Equation (S8) shows $\theta$ is a function of OD ($\alpha$) and one-photon detuning ($\Delta$). According to $t_1$ and $r_1$ (or $t_2$ and $r_2$) in Eq. (S14), the split ratio is related to $\theta$ as

$$s = \frac{1}{2}\left(1 - \frac{2e^{-A}}{1 + e^{-2A}}\cos\theta\right). \tag{S19}$$

One can immediately see that $\theta \approx \pi$ makes $s \to 1$ under a small $A$ (i.e., a large $\alpha$), and $\theta = \pi/2$ exactly makes $s = 0.5$. Based on Eq. (S14), the total transmission of FBS is

$$T = \frac{1 + e^{-2A}}{2}. \tag{S20}$$

The ideal BS must have $\phi_1 + \phi_2 = \pi$ in Eq. (S13) [15, 16]. Corresponding to $\hat{V}$ in Eq. (S14) of $\phi_1 = \phi_2 = \phi$ and the split ratio of $s$, the operator $\hat{U}$ of ideal BS is given by

$$\hat{U} = \begin{bmatrix} \sqrt{1-s} & i\sqrt{s} \\ i\sqrt{s} & \sqrt{1-s} \end{bmatrix}.$$

With $\hat{V}$ in Eq. (S14) and the above $\hat{U}$, Eq. (S12) becomes

$$F = \frac{1}{4T}\Big[(1 + e^{-2A}) + 2(1 - 2s)e^{-A}\cos\theta \tag{S21}$$
$$+2\sqrt{s(1-s)}\sqrt{(1 + e^{-2A})^2 - 4e^{-2A}\cos^2\theta}\,\sin\left(\frac{\phi}{2}\right)\Big].$$

### B. 50/50 Frequency Beam Splitter

We again consider the case that the ground-state decoherence rate in the system is negligible, i.e., $\gamma = 0$. The 50/50 FBS has $\theta = \pi/2$, making $\cos\theta = 0$ and $s = 0.5$, as indicated by Eq. (S19). Using $\cos\theta = 0$ in Eq. (S21), we find that the fidelity of 50/50 FBS is

$$F = \frac{1}{2} + \frac{1}{2}\sin\left(\frac{\phi}{2}\right). \tag{S22}$$

Since the value of $\alpha$ (OD) in our experiment was large as compared with $\theta$, $A \approx 2\theta^2/\alpha = \pi^2/(2\alpha) \ll 1$ in Eq. (S17). We set $\theta = \pi/2$ in Eq. (S18) to get $\sin(\phi/2)$, and utilize $A \ll 1$ to obtain

$$F = \frac{1}{2} + \frac{e^{-A}}{1 + e^{-2A}} \approx 1 - \frac{A^2}{4} \approx 1 - \frac{\pi^4}{16\alpha^2}. \tag{S23}$$

Using $A \ll 1$ in Eq. (S20),

$$T \approx 1 - A = 1 - \frac{\pi^2}{2\alpha}. \quad \text{(S24)}$$

Therefore, a larger OD not only results in a lower loss, but also makes the fidelity better.

### C. Realistic Frequency Beam Splitter

In reality, the ground-state decoherence rate $\gamma$ in the experimental system was not negligible. A nonzero $\gamma$ makes two inputs of the FWM-based FBS produce different split ratios, i.e., $r_1^2/(t_1^2 + r_1^2) \neq r_2^2/(t_2^2 + r_2^2)$, and different phases, i.e., $\phi_1 \neq \phi_2$. Corresponding to the general expression of $\hat{V}$ in Eq. (S13) of nonzero $\Delta\phi = \phi_1 - \phi_2$, the operator $\hat{U}$ of ideal 50/50 BS is given by

$$\hat{U} = \frac{1}{\sqrt{2}} \begin{bmatrix} 1 & e^{i(\pi-\Delta\phi)/2} \\ e^{i(\pi+\Delta\phi)/2} & 1 \end{bmatrix}. \quad \text{(S25)}$$

The above expressions of phases in the off-diagonal terms ensure that the ideal BS has $\phi_1 + \phi_2 = \pi$. With $\hat{V}$ in Eq. (S13) and the above $\hat{U}$, the fidelity in Eq. (S12) becomes

$$F = \frac{1}{2} + \frac{\bar{t}\bar{r}}{T} \sin\left(\frac{\phi}{2}\right), \quad \text{(S26)}$$

where $\bar{t} = (t_1 + t_2)/2$, $\bar{r} = (r_1 + r_2)/2$, $T = \bar{t}^2 + \bar{r}^2$, and $\phi = \phi_1 + \phi_2$.

## VI. DETERMINATION OF THE PHASE OF FREQUENCY BEAM SPLITTER WITH HOMI

The phase $\phi$ in Eq. (S21) is the sum of the phase difference between the reflected and transmitted waves of input 1, $\phi_1$, and that of input 2, $\phi_2$, in Eq. (S13), i.e., $\phi = \phi_1 + \phi_2$. The following example illustrates how the measurement of $g^{(2)}$ in the Hong-Ou-Mandel interference (HOMI) can determine $\phi$. A beam splitter (BS) is represented by the matrix in Eq. (S13). In the HOMI, two single photons of the Fock state are sent to the two input ports of BS. The value of $g^{(2)}$ of the two output ports of BS is defined by

$$g^{(2)} \equiv \frac{\langle N_1 N_2 \rangle}{\langle N_1 \rangle \langle N_2 \rangle}, \quad \text{(S27)}$$

where $\langle N_1 \rangle$ or $\langle N_2 \rangle$ is the photon count of each output mode, and $\langle N_1 N_2 \rangle$ is the photon-photon coincidence count between the two output modes. Because of the energy (photon number) conservation, $\langle N_1 \rangle = t_1^2 + r_2^2$ and $\langle N_2 \rangle = t_2^2 + r_1^2$, where $t_1$ ($t_2$) and $r_1$ ($r_2$) are the transmission and reflection coefficients of input 1 (input 2). The major outcomes of the BS correspond to the following two-mode wave functions of $t_1 t_2 |1, 1\rangle$, $t_1 r_2 e^{i\phi_2} \sqrt{2} |2, 0\rangle$, $t_2 r_1 e^{i\phi_1} \sqrt{2} |0, 2\rangle$, and $r_1 r_2 e^{i\phi} |1, 1\rangle$, where the first and second quanta represent photon numbers in two output modes. Only the wave functions of $|1, 1\rangle$ can contribute to $\langle N_1 N_2 \rangle$, which is equal to $(t_1 t_2 + r_1 r_2 e^{-i\phi})(t_1 t_2 + r_1 r_2 e^{i\phi})$, and those of $|2, 0\rangle$ and $|0, 2\rangle$ do not make any contribution. Other possible output wave functions are proportional to $|1, 0\rangle$, $|0, 1\rangle$, and $|0, 0\rangle$, which do not contribute to $\langle N_1 N_2 \rangle$, either. Once knowing $\langle N_1 \rangle$, $\langle N_2 \rangle$, and $\langle N_1 N_2 \rangle$ [16], we obtain

$$g^{(2)} = \frac{t_1^2 t_2^2 + r_1^2 r_2^2 + 2 t_1 t_2 r_1 r_2 \cos\phi}{(t_1^2 + r_2^2)(t_2^2 + r_1^2)}. \quad \text{(S28)}$$

Therefore, given the BS's $t_1$, $r_1$, $t_2$, and $r_2$, one can determine $\phi$ from the value of $g^{(2)}$ as demonstrated by the above equation.

A 50/50 BS has $t_1 = r_1 = t_2 = r_2$. Based on Eq. (S28), $g^{(2)} = (1 + \cos\phi)/2$ revealing that the two-photon event corresponding to $t_1 t_2 |1, 1\rangle$ (both input photons transmit through the BS) interferes with that corresponding to $r_1 r_2 e^{i\phi} |1, 1\rangle$ (both are reflected by the BS). An ideal 50/50 BS further has $\phi = \pi$ [15, 16], making $g^{(2)} = 0$ which is exactly the consequence that the interference is completely destructive. With two Fock-state single photons at two input ports of the ideal BS in the HOMI, it is well known that both photons always emerge together at one of the output ports (corresponding to $|2, 0\rangle$ or $|0, 2\rangle$) as depicted in Fig. 1(c), resulting in $g^{(2)} = 0$ [17, 18]. With two coherent-state single photons, one can also show that the HOMI of ideal 50/50 BS results in $g^{(2)} = 0.5$ [19–21].

## VII. HOMI MEASUREMENT WITH COHERENT-STATE PHOTONS

In this section, we will derive the value of $g^{(2)}$ in the Hong-Ou-Mandel interference (HOMI) of a realistic beam splitter (BS) with coherent-state light. To make the theoretical situation consistent with the experimental condition of our HOMI measurement, we consider that the phases of the two input coherent states are completely uncorrelated, and the mean photon numbers of the two states are the same. Equation (S13) represents the operator of realistic BS. Two coherent states $|\alpha\rangle$ and $|\alpha e^{i\xi}\rangle$ are incident to inputs 1 and 2 of the BS, respectively, where $\xi$ is the relative phase between the two states. Since the two coherent states are phase-uncorrelated, we will average $\xi$ over all phases later.

In Eq. (S13), the transmission and reflection coefficients of input 1 (or input 2) of the BS are $t_1$ (or $t_2$) and $r_1$ (or $r_2$), respectively, and the phase difference between the reflected and transmitted light is $\phi_1$ (or $\phi_2$). Thus, the two wave functions emerging at output 1 and 2 of the

BS are given by

$$\psi_1 = |t_1\alpha + (r_2 e^{i\phi_2})\alpha e^{i\xi}\rangle_1 = \left|[t_1 + r_2 e^{i(\phi_2+\xi)}]\alpha\right\rangle_1, \quad \text{(S29)}$$

$$\psi_2 = |(r_1 e^{i\phi_1})\alpha + t_2\alpha e^{i\xi}\rangle_2 = \left|(r_1 e^{i\phi_1} + t_2 e^{i\xi})\alpha\right\rangle_2, \quad \text{(S30)}$$

where the subscripts 1 and 2 indicate the output modes 1 and 2. Let's denote $\langle N_1\rangle$ and $\langle N_2\rangle$ as the photon counts of outputs 1 and 2 of the BS, and $\langle N_1 N_2\rangle$ as the photon-photon coincidence count between the two outputs. The value of $g^{(2)}$ is defined by

$$g^{(2)} \equiv \frac{\langle N_1 N_2\rangle}{\langle N_1\rangle\langle N_2\rangle}. \quad \text{(S31)}$$

With $\psi_1$ and $\psi_2$, we can evaluate $\langle N_1\rangle$ and $\langle N_2\rangle$ with the photon number operators $a_1^\dagger a_1$ and $a_2^\dagger a_2$ in the followings:

$$\langle N_1\rangle = \frac{1}{2\pi}\int_0^{2\pi} d\xi\ \psi_1^\dagger(a_1^\dagger a_1)\psi_1 = (t_1^2 + r_2^2)|\alpha|^2, \quad \text{(S32)}$$

$$\langle N_2\rangle = \frac{1}{2\pi}\int_0^{2\pi} d\xi\ \psi_2^\dagger(a_2^\dagger a_2)\psi_2 = (r_1^2 + t_2^2)|\alpha|^2. \quad \text{(S33)}$$

The two-mode wave function at the output, $\psi_{12}$, is the direct product of $\psi_1$ and $\psi_2$, i.e., $\psi_{12} = \psi_1 \otimes \psi_2$. Hence, the value of $\langle N_1 N_2\rangle$ is given by

$$\begin{aligned}\langle N_1 N_2\rangle &= \frac{1}{2\pi}\int_0^{2\pi} d\xi\ \psi_{12}^\dagger(a_1^\dagger a_1 a_2^\dagger a_2)\psi_{12} \quad \text{(S34)}\\ &= \left[(t_1^2 + r_2^2)(r_1^2 + t_2^2) + 2t_1 t_2 r_1 r_2 \cos(\phi_1 + \phi_2)\right]|\alpha|^4.\end{aligned}$$

Knowing the values of $\langle N_1\rangle$, $\langle N_2\rangle$, and $\langle N_1 N_2\rangle$, we obtain

$$g^{(2)} = 1 + \frac{2t_1 t_2 r_1 r_2}{(t_1^2 + r_2^2)(t_2^2 + r_1^2)}\cos\phi, \quad \text{(S35)}$$

where $\phi = \phi_1 + \phi_2$. Both $g^{(2)}$ and fidelity, $F$, are related to $\phi$ as demonstrated by the above equation and Eq. (S26). Therefore, given $t_1$, $r_1$, $t_2$, and $r_2$ of a realistic BS, one can determine the fidelity of this BS from the value of $g^{(2)}$ in the HOMI measurement.


[1] Y.-W. Lin, H.-C. Chou, P. P. Dwivedi, Y.-C. Chen, and I. A. Yu, *Using a pair of rectangular coils in the MOT for the production of cold atom clouds with large optical density*, Opt. Express **16**, 3753 (2008).

[2] M.-J. Lee, J. Ruseckas, C.-Y. Lee, V. Kudriăsov, K.-F. Chang, H.-W. Cho, G. Juzeliūnas, and I. A. Yu, *Experimental demonstration of spinor slow light*, Nat. Commun. **5**, 5542 (2014).

[3] Y.-H. Chen, M.-J. Lee, I.-C. Wang, and I. A. Yu, *Fidelity of electromagnetically-induced-transparency-based optical memory*, Phys. Rev. A **88**, 023805 (2013).

[4] S.-W. Su, Y.-H. Chen, S.-C. Gou, T.-L. Horng, and I. A. Yu, *Dynamics of slow light and light storage in a Doppler-broadened electromagnetically-induced-transparency medium: A numerical approach*, Phys. Rev. A **83**, 013827 (2011).

[5] S.-W. Su, Y.-H. Chen, S.-C. Gou, and I. A. Yu, *An effective thermal-parametrization theory for the slow-light dynamics in a Doppler-broadened electromagnetically induced transparency medium*, J. Phys. B **44**, 165504 (2011).

[6] M. Jain, H. Xia, G. Y. Yin, J. Merriam, and S. E. Harris, *Efficient Nonlinear Frequency Conversion with Maximal Atomic Coherence*, Phys. Rev. Lett. **77**, 4326 (1996).

[7] Y.-H. Chen, M.-J. Lee, I.-C. Wang, S. Du, Y.-F. Chen, Y.-C. Chen, and I. A. Yu, *Coherent Optical Memory with High Storage Efficiency and Large Fractional Delay*, Phys. Rev. Lett. **110**, 083601 (2013).

[8] Y.-F. Hsiao, P.-J. Tsai, H.-S. Chen, S.-X. Lin, C.-C. Hung, C.-H. Lee, Y.-H. Chen, Y.-F. Chen, I. A. Yu, and Y.-C. Chen, *Highly Efficient Coherent Optical Memory Based on Electromagnetically Induced Transparency*, Phys. Rev. Lett. **120**, 183602 (2018).

[9] C.-K. Chiu, Y.-H. Chen, Y.-C. Chen, I. A. Yu, Y.-C. Chen, and Y. F. Chen, *Low-light-level four-wave mixing by quantum interference*, Phys. Rev. A **89**, 023839 (2014).

[10] C.-Y. Lee, B.-H. Wu, G. Wang, Y.-F. Chen, Y.-C. Chen, and I. A. Yu, *High conversion efficiency in resonant four-wave mixing processes*, Opt. Express **24**, 1008 (2016).

[11] M. Fleischhauer, A. Imamoglu, and J. Marangos, *Electromagnetically induced transparency: Optics in coherent media*, Rev. Mod. Phys. **77**, 633 (2005).

[12] D. B. Uskov, L. Kaplan, A. M. Smith, S. D. Huver, and J. P. Dowling, *Maximal success probabilities of linear-optical quantum gates*, Phys. Rev. A **79**, 042326 (2009).

[13] S. Rahimi-Keshari, M. A. Broome, R. Fickler, A. Fedrizzi, T. C. Ralph, and A. G. White, *Direct characterization of linear-optical networks*, Opt. Express **21**, 13450 (2013).

[14] H.-H. Lu, J. M. Lukens, N. A. Peters, O. D. Odele, D. E. Leaird, A. M. Weiner, and P. Lougovski, *Electro-Optic Frequency Beam Splitters and Tritters for High-Fidelity Photonic Quantum Information Processing*, Phys. Rev. Lett. **120**, 030502 (2018).

[15] S. M. Barnett, J. Jeffers, and A. Gatti, *Quantum optics of lossy beam splitters*, Phys. Rev. A **57**, 2134 (1998).

[16] R. Uppu, T. A. W. Wolterink, T. B. H. Tentrup, and P. W. H. Pinkse, *Quantum optics of lossy asymmetric beam splitters*, Opt. Express **24**, 16440 (2016).

[17] C. K. Hong, Z. Y. Ou, and L. Mandel, *Measurement of*

*Subpicosecond Time Intervals between Two Photons by Interference*, Phys. Rev. Lett. **59**, 2044 (1987).

[18] T. B. Pittman, D. V. Strekalov, A. Migdall, M. H. Rubin, A. V. Sergienko, and Y. H. Shih, *Can Two-Photon Interference be Considered the Interference of Two Photons?*, Phys. Rev. Lett. **77**, 1917 (1996).

[19] J. G. Rarity, P. R. Tapster, and R. Loudon, *Non-classical interference between independent sources*, J. Opt. B: Quantum Semiclass. Opt. **7**, S171 (2005).

[20] Y.-S. Kim, O. Slattery, P. S. Kuo, and X. Tang, *Conditions for two-photon interference with coherent pulses*, Phys. Rev. A **87**, 063843 (2013).

[21] H. Chen, X.-B. An, J. Wu, Z.-Q. Yin, S. Wang, W. Chen, and Z.-F. Han, *Hong-Ou-Mandel interference with two independent weak coherent states*, Chin. Phys. B **25**, 020305 (2016).
